# Supplementary material for: Preserving Generalization of Language models in Few-shot Continual Relation Extraction
Source: arXiv:2410.00334 source file (2024-10-01)
Supplement: Supplementary file 1 [file 7.1-appendix_baselinedetailed.tex]

\subsection{Prototype Based Classification Module}
Similar to recent advancements in prototype-based relation classification (\textbf{[ConPL]}), we adopt a similar strategy.

\begin{figure}[ht]
  \includegraphics[width=\columnwidth]{latex/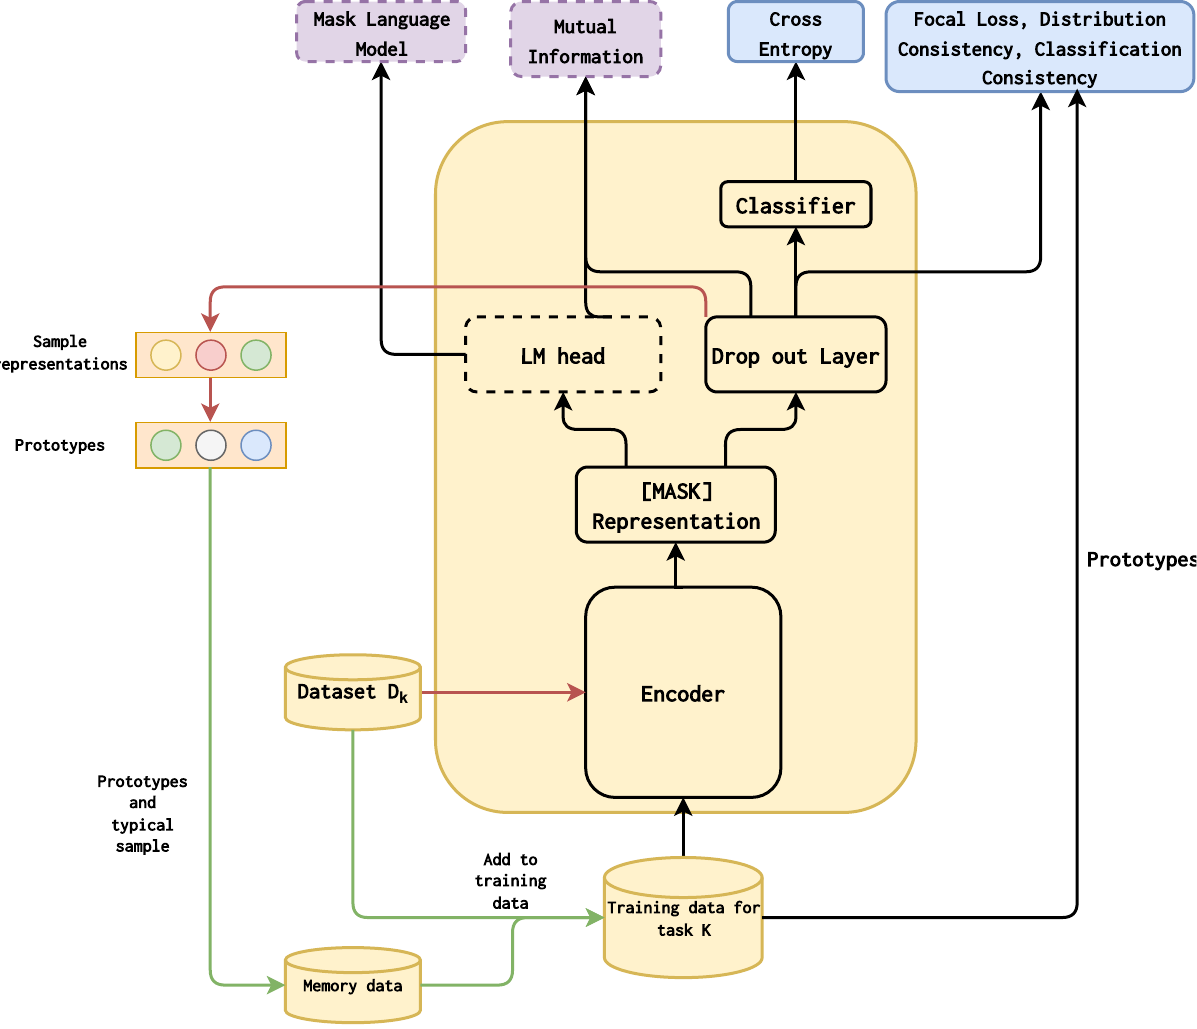}
  \caption{Framework - ConPL}
  \label{fig:framwork_conpl}
\end{figure}

\noindent \textbf{Encoder}. Our approach leverages a pre-trained BERT model (\textbf{[BERT]}) as the encoder, denoted by parameters $\theta$. Given a sentence x containing a head entity $e_{h}$ and a tail entity $e_{t}$, we aim to capture the relational representation between these entities within the sentence. We use a specific input sequence $x_{input} = \{[CLS], e_{h}, [MASK], e_{t}, [SEP], x, [SEP]\}$ . and then encode the input sequence by the encoder to obtain the contextualized representation. Here we use the vector representation of the special token [MASK] as the relational representation.

$$h_{MASK} = f_{\theta}(x_{input})$$

\noindent \textbf{Initializing temporary prototypes of new classes:} When training on new task (e.g. the $k^{\text{th}}$ task) to learn novel relations, we employ all samples associated with each new relationship to construct prototypical representations for their corresponding classes. 
In particular, we encode all samples within the training set $D_{\text{train}}^k$, followed by the application of an aggregation operator (e.g., averaging) to combine the embeddings of samples belonging to the same class. Thus, the prototypical representation $\mathbf{p}_j$ for class $j$ can be formulated as:

\begin{equation}
\mathbf{p}_j = \frac{1}{|D_j^k|} \sum_{(x_i, y_i) \in D_j^k} f_\theta(x_i)
\end{equation}

where $D_j^k = \{(x_i, y_i) \mid (x_i, y_i) \in D_{\text{train}}^k, y_i = r_j\}$, $|D_j^k|$ denotes the number of samples , and $\mathbf{p}_j$ represents the prototypical representation of relation $r_j$ $(r_j \in R^k)$. Therefore, the temporary prototypes of the current new task are given by $\tilde{P}^k = \bigcup_{r_j \in R^k} \mathbf{p}_j$. Incorporating the pre-existing relation prototypes $\hat{P}^{k-1}$ stored in memory, we obtain the collection of present prototypes $\bar{P}^k = \hat{P}^{k-1} \cup \tilde{P}^k$, which represent all encountered classes up to the $k^{th}$ task.
% \footnote{$\tilde{P}^k$ refers to the temporary prototypes of the $k$-th task and $P^k$ refers to the prototypes of the $k$-th task stored in memory. $\bar{P}^k$ refers to the prototypes of the previous $k$ task that contain the prototypes from memory for the previous $k-1$ tasks as well as the temporary prototypes for the $k$-th task. Additionally, $\hat{P}^k$ refers to the prototypes of the previous $k$ task stored in memory.}

% \noindent \textbf{Prototype classifier with experience replay:} \\
\textbf{Classification Loss:} To facilitate the learning of new relations while preserving existing relation knowledge, we employ experience replay to train the model on the updated training dataset $\bar{D}_{\text {train }}^k=$ $D_{\text {train }}^k \cup \hat{S}^{k-1}$, comprising the training instances from the current $k$-th task with those from the preceding $k-1$ tasks stored in memory. The relation distribution for each sample $x_i$ is then computed as:
$$
p\left(r_i \mid x_i\right)=\frac{\exp \left(d\left(f_\theta\left(x_i\right), \mathbf{p}_i\right)\right)}{\sum_{l=1}^{\left|\bar{R}^k\right|} \exp \left(d\left(f_\theta\left(x_i\right), \mathbf{p}_l\right)\right)}
$$
where $d(., .)$ represents the distance measurement formula by the cosine similarity, $\mathbf{p}_l$ is the prototypical representation of $r_l\left(r_l \in \bar{R}^k\right)$ in $\bar{P}^k$, and $\left|\bar{R}^k\right|$ is the number of known relations up to $k^{th}$ task.

The cross-entropy loss $\mathcal{L}_{c e}$ for classification is calculated in a distance measurement way.
$$
\mathcal{L}_{c e}=-\sum_{\left(x_i, y_i\right) \in \bar{D}_{\text {train }}^k} \log p\left(r_i \mid x_i\right)
$$

\textbf{Classification Consistency Loss:} To reactivate prior relational knowledge, we introduce the classification consistency loss $\mathcal{L}_{cc}$, which emphasizes the consistent correlation between the features of each sample in $\hat{S}^{k-1}$ and the corresponding prototypical representation in $\hat{P}^{k-1}$, leveraging the current memory.
$$
\mathcal{L}_{c c}=\sum_{\left(x_i, y_i\right) \in \hat{S}^{k-1}}\left\|f_\theta\left(x_i\right)-\mathbf{p}_i\right\|
$$

\textbf{Distinguishing similar prototypes using Focal Loss:} Taking into account the relationship between newly introduced relations and those from previous tasks (for instance, the relation "mother" in the new task and previous relations such as "father" or "spouse" belonging to closely related categories), our objective is to differentiate between similar relations. 
Specifically, when examining sample $x_i$, with relation $r_i$  corresponding to prototype $\mathbf{p}_i$, we utilize two strategies for selecting the set of similar prototypes.
\begin{enumerate}
    \item We first acquire the most similar negative prototype, which represents the prototype associated with the relation most likely to be misinterpreted as:
    \begin{equation}
        \mathbf{p}_s^* =\underset{\mathbf{p}_s, \mathbf{p}_s \neq \mathbf{p}_i}{argmax}\left(d\left(f_\theta\left(x_i\right), \mathbf{p}_s\right)\right) \nonumber
    \end{equation}
    \item 
    
\end{enumerate}

Specifically, we start by obtaining the most similar negative prototype $\mathbf{p}_i^{m n}=\operatorname{argmax}\left(d\left(f_\theta\left(x_i\right), \mathbf{p}_s\right)\right)$ for each sample $x_i$, which is the prototype of the most likely relation of miscalculation. Next, we set a threshold $\alpha$ and automatically screen some confusing negative prototypes $\hat{\mathbf{p}}_i^{s n}=$ $\left\{\mathbf{p}_i^{s n} \mid d\left(f_\theta\left(x_i\right), \mathbf{p}_i\right)-d\left(f_\theta\left(x_i\right), \mathbf{p}_i^{s n}\right)<\alpha\right\} \quad$ that include prototypes that are the most similar to the prototype $\mathbf{p}_i$ with the target relation. Here $\mathbf{p}_s$ and $\mathbf{p}_i^{s n}$ refer to any prototype other than $\mathbf{p}_i$, so $\mathbf{p}_s \neq \mathbf{p}_i$ and $\mathbf{p}_i^{s n} \neq \mathbf{p}_i$. The distribution of $x_i$ is computed for distinguishing similar classes.
$$
p_s\left(r_i \mid x_i\right)=\frac{\exp \left(d\left(f_\theta\left(x_i\right), \mathbf{p}_i\right)\right)}{\sum_{l=1}^{\left|P_i^{s i m}\right|} \exp \left(d\left(f_\theta\left(x_i\right), \mathbf{p}_l\right)\right)}
$$
where $P_i^{s i m}=\left[\mathbf{p}_i ; \mathbf{p}_i^{m n} ; \hat{\mathbf{p}}_i^{s n}\right]$ represents the set of prototypes similar to the output feature of $x_i$ and $\left|P_i^{s i m}\right|$ is the number.

Therefore, we adopt the focal loss to alleviate the difficulty in predicting similar classes.
$$
\mathcal{L}_{f c}=-\sum_{\left(x_i, y_i\right) \in \bar{D}_{\text {train }}^k} \log p_s\left(r_i \mid x_i\right)
$$
\subsection{ Memory-Enhanced Module}

Compared to previous memory-based methods (Han et al., 2020; Cui et al., 2021; Qin and Joty, 2022), we add prototypical representations into the episodic memory for enriching the old relations. So the memory of our model is separated into two parts: the Sample Memory $\hat{S}^k$, which is used to store samples with class labels, and the Prototype Memory $\hat{P}^k$, which is used to store feature embeddings of class prototypes.

For the sample memory, we calculate the prototypical representation of each relation in the current task $\mathcal{T}^k$ based on Eq (2), and then select some closest samples as the typical samples to store them in $S^k$, where each relation of $\mathcal{T}^k$ only stores one typical sample. During training, prototypical representations computed by all relation samples can be unstable. Therefore, once the typical samples are determined, we use the feature representations of the selected typical samples to update prototypical representations of the current task and store their feature representations in prototype memory $P^k$ after $\mathcal{T}^k$ is trained.
4.3 Consistent Learning Module

Considering the unbalanced distribution of new relations and old ones in the training dataset $\bar{D}_{\text {train }}^k$, we add an extended training step that solely focuses on the memory $\mathcal{M}$ that helps to balance the learning of all known relations and distinguish new and old relations. Therefore, we propose the distribution consistency loss $\mathcal{L}_{d c}$ via computing the consistent constraint between the sample distribution and the prototype distribution.
$$
\mathcal{L}_{d c}=\sum_{\left(x_i, y_i\right) \in \hat{S}^k}\left\|d\left(f_\theta\left(x_i\right), \hat{P}^k\right)-d\left(\mathbf{p}_i, \hat{P}^k\right)\right\|
$$

\begin{figure}[ht]
  \includegraphics[width=\columnwidth]{latex/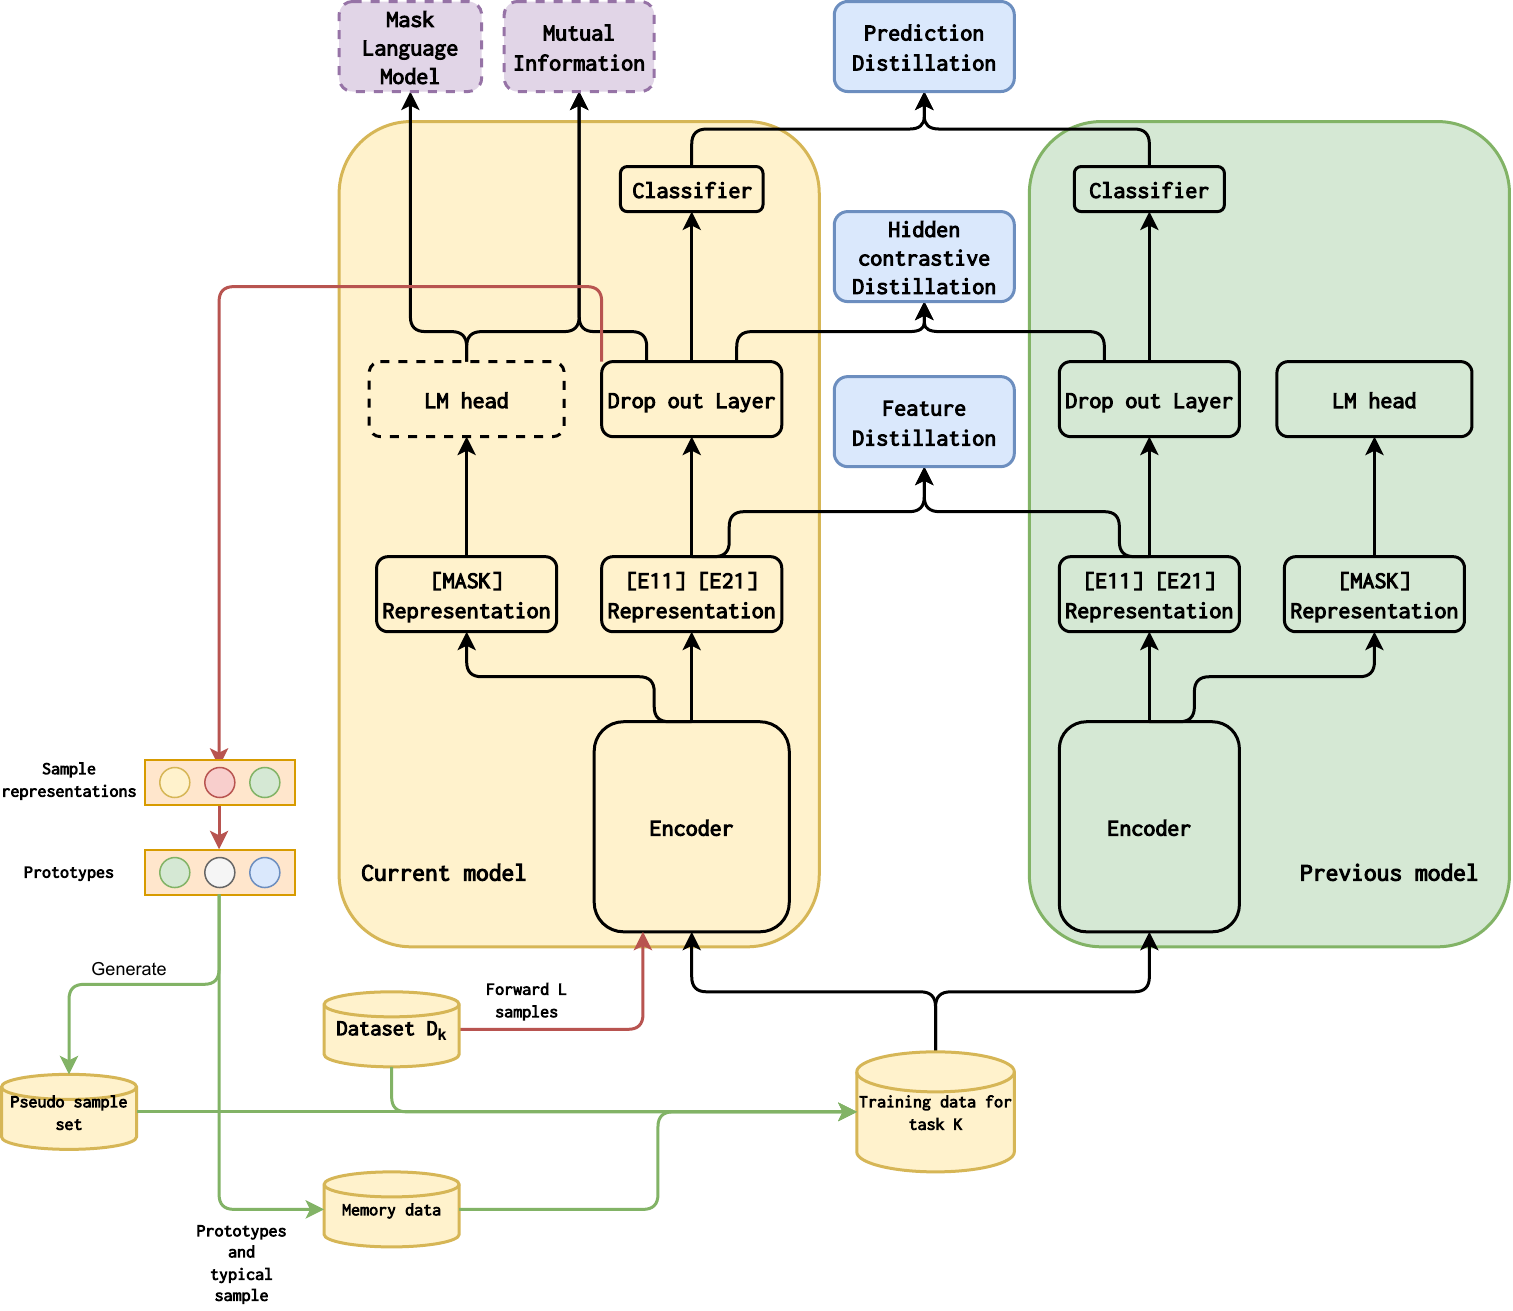}
  \caption{Framework - SCKD}
  \label{fig:framwork_sckd}
\end{figure}

\subsection{SCKD}
3.2 Our Framework

Algorithm 1 shows the end-to-end training for task $T_j$, with the model $\Phi_{j-1}$ previously trained. Following the memory-based methods for continual learning (Lopez-Paz and Ranzato, 2017; Chaudhry et al., 2019), we use a memory $\tilde{M}_{j-1}$ to preserve a few samples in all previous tasks $\left\{T_1, \ldots, T_{j-1}\right\}$.
1. Initialization (Line 1). The current model $\Phi_j$ inherits the parameters of $\Phi_{j-1}$, except for $\Phi_1$ randomly initialized. We adapt $\Phi_j$ on $D_j$ to learn the knowledge of new relations in $T_k$.
2. Prototype generation (Lines 2-6). Inspired by (Han et al., 2020; Cui et al., 2021), we apply the k-means algorithm to select $L$ typical samples from $D_j$ for every relation $r \in R_j$, which constitute a memory $M_r$. The memory for the current task is $M_j=\bigcup_{r \in R_j} M_r$, and the overall memory for all observed relations until now is $\tilde{M}_j=\tilde{M}_{j-1} \cup M_j$. Then, we generate a prototype $\mathbf{p}_r$ for each $r \in \tilde{R}_j$.
3. Data augmentation (Line 7). To cope with the scarcity of samples, we conduct bidirectional data augmentation between $D_j$ and $\tilde{M}_j$. By measuring the similarity between entities in samples, we generate an augmented dataset $D_j^*$ and an augmented memory $\tilde{M}_j^*$ by mutual replacement between similar entities.
4. Serial Contrastive Knowledge Distillation (Lines 8-10). We construct a set of pseudo samples based on the prototype set. Then, we carry out serial contrastive knowledge distillation with the pseudo samples on $D_j^*$ and on $\tilde{M}_j^*$, respectively, making the sample representations in different relations distinguishable and preserve the prior knowledge for identifying the relations in previous tasks well.

We detail the procedure in the subsections below.
3.3 Initialization for New Task

To adapt the model for the new task $T_j$, we perform a simple multi-classification task on dataset $D_j$.

Specifically, for a sample $x$ in $T_j$, we use special tokens $\left[E_1\right]$ and $\left[E_2\right]$ to denote the start positions of Algorithm 1: Training procedure for $T_j$
Input: $\Phi_{j-1}, \tilde{R}_{j-1}, \tilde{M}_{j-1}, D_j, R_j$
Output: $\Phi_j, \tilde{M}_j$
initialize $\Phi_j$ from $\Phi_{j-1}$, and adapt it on $D_j$;
$\tilde{M}_j \leftarrow \tilde{M}_{j-1}$;
foreach $r \in R_j$ do
pick $L$ samples in $D_j$, and add into $\tilde{M}_j$;
$\tilde{R}_j \leftarrow \tilde{R}_{j-1} \cup R_j$
generate prototype set $\tilde{P}_j$ based on $\tilde{M}_j$;
generate augmented dataset $D_j^*$ and memory
$\tilde{M}_j^*$ by mutual replacement;
generate pseudo sample set $\tilde{S}_j$ based on $\tilde{P}_j$;
update $\Phi_j$ by serial contrast. knowl. distill.
on $D_j^*, \tilde{S}_j ; \quad / /$ re-train current task
update $\Phi_j$ by serial contrast. knowl. distill.
on $\tilde{M}_j^*, \tilde{S}_j ; \quad / /$ memory replay
two entities in $x$, respectively. Then, we obtain the representations of special tokens using the BERT encoder (Devlin et al., 2019). Next, the feature of sample $x$, denoted by $\mathrm{f}_x$, is defined as the concatenation of token representations of $\left[E_1\right]$ and $\left[E_2\right]$. We obtain the hidden representation $\mathbf{h}_x$ of $x$ as
$$
\mathbf{h}_x=\mathrm{LN}\left(\mathbf{W} \operatorname{Dropout}\left(\mathbf{f}_x\right)+\mathbf{b}\right),
$$
where $\mathbf{W} \in \mathbb{R}^{d \times 2h}$ and $\mathbf{b} \in \mathbb{R}^d$ are two trainable parameters, $d$ is the dimension of hidden layers, $h$ is the dimension of BERT hidden representations, $\mathrm{LN}(\cdot)$ is the layer normalization operation.

Finally, based on $\mathbf{h}_x$, we use the linear softmax classifier to predict the relation label. The classification loss, $\mathcal{L}_{\text {csf }}$, is defined as
$$
\mathcal{L}_{\text {csf }}=-\frac{1}{\left|D_j\right|} \sum_{x \in D_j} \sum_{r=1}^{\left|R_j\right|} y_{x, r} \cdot \log P_{x, r},
$$
where $y_{x, r} \in\{0,1\}$ indicates whether $x$ 's true label is $r . P_{x, r}$ denotes the $r$-th entry in $x$ 's probability distribution calculated by the classifier.
3.4 Prototype Generation

After the initial adaption above, we pick $L$ typical samples for each relation $r \in R_j$ to form memory $M_r$. We leverage the k-means algorithm upon the hidden representations of $r$ 's samples, where the number of clusters equals the number of samples that need to be stored for representing $r$. Then, in each cluster, the sample closest to the centroid is chosen as one typical sample.
To obtain the prototype $\mathbf{p}_r$ for $r$, we average the hidden representations of $L$ typical samples in $M_{\mathrm{r}}$ :
$$
\mathbf{p}_r=\frac{1}{L} \sum_{x \in M_r} \mathbf{h}_x .
$$

The prototype set $\tilde{P}_j$ stores the prototypes of all relations in $\tilde{R}_j$, i.e., $\tilde{P}_j=\cup_{r \in \tilde{R}_j}\left\{\mathbf{p}_r\right\}$.
3.5 Bidirectional Data Augmentation

For a sample $x$ in $D_j$ or $\tilde{M}_j$, the token representations of $\left[E_1\right]$ and $\left[E_2\right]$ generated by BERT are used as the representations of corresponding entities. We obtain the entity representations from all samples and calculate the cosine similarity between the representations of any two different entities. Once the similarity exceeds a threshold $\tau$, we replace each of the two entities in the original sample with the other entity. Our intuition is that one certain entity in a sentence is replaced by its close entity with everything else unchanged, the relation represented by the sentence is unlikely to change much. For example, "The route crosses the Minnesota River at the Cedar Avenue Bridge." and "The route crosses the River MNR at the Cedar Avenue Bridge." have the same relation "crosses". We assign the same relation label to the new samples as their original samples and store them together as the augmented dataset $D_j^*$ and the augmented memory $\tilde{M}_j^*$.
3.6 Serial Contrastive Knowledge Distillation

Knowledge distillation (Hinton et al., 2015; Cao et al., 2020) has demonstrated its effectiveness in transferring knowledge. In this paper, we propose a serial contrastive knowledge distillation method to leverage the knowledge from the previous RE model to guide the training of the current model. The procedure of serial contrastive knowledge distillation is depicted in Figure 2. We detail it below.

Feature distillation. In this step, we expect the encoder of the current model to extract similar features with the previous model. For a sample $x$, let $\mathbf{f}_x^{j-1}$ and $\mathbf{f}_x^j$ be $x$ 's features extracted by the previous model $\Phi_{j-1}$ and the current model $\Phi_j$, respectively. We propose a feature distillation loss to enforce the extracted features unbiased towards new relations:
$$
\mathcal{L}_{\mathrm{fd}}=\frac{1}{\left|\tilde{M}_j^*\right|} \sum_{x \in \tilde{M}_j^*}\left(1-\left(\mathbf{f}_x^{j-1}\right)^{\top} \mathbf{f}_x^j\right) .
$$

\subsection{CPL}

The Continual Prompt Learning (CPL) framework addresses the challenges of catastrophic forgetting and overfitting in Continual Few-Shot Relation Extraction (CFRE). It leverages prompt learning to enhance PLMs' ability to retain knowledge across tasks and introduces a novel margin-based contrastive learning approach for improved generalization. CPL have the following key concepts.

Contrastive Prompt Learning (CPL) \textbf{[CITE]} is an FCRE framework that leverages prompt learning and a novel margin-based contrastive learning approach for improved generalization. CPL have the following key concepts.

\textbf{Prompt Representation} : CPL employs a hybrid prompt template combining entity information and learnable tokens. This semi-automated approach guides PLMs to effectively capture task-specific knowledge, converting RE into a cloze-style task.

CPL utilizes a semi-automated continuous prompt template, combining entity information and learnable tokens , for an input sentence $x$ with two entities $e_h$ and $e_t$, the template is as follows:
$$
\begin{aligned}
T(\boldsymbol{x})= & \boldsymbol{x} \cdot\left[v_{0: n_0-1}\right] \boldsymbol{e}_{\boldsymbol{h}}\left[v_{n_0: n_1-1}\right][\text { MASK }] \\
& {\left[v_{n_1: n_2-1}\right] \boldsymbol{e}_{\boldsymbol{t}}\left[v_{n_2: n_3-1}\right] . }
\end{aligned}
$$
where $\left[v_i\right]$ refers to the $i$-th learnable continuous token, and $n_i$ is the length of token phrases. The [MASK] in the template as the representation of the relation between $e_h$ and $e_t$.

Given a encoding model $E$ and a templated sentence $T(\boldsymbol{x})$ as input, The input sentence with the applied template, $T(\boldsymbol{x})$, is then encoded into continuous vectors:

\begin{align}
& E_{m b}(T(\boldsymbol{x}))=e(\boldsymbol{x}), h_0, \ldots, h_{n_0-1}, e\left(\boldsymbol{e}_{\boldsymbol{h}}\right) \text {, } \nonumber \\
& h_{n_0}, \ldots, h_{n_1-1}, e([\text { MASK }]), h_{n_1}, \nonumber \\
& \ldots, h_{n_2-1}, e\left(\boldsymbol{e}_{\boldsymbol{t}}\right), h_{n_2}, \ldots, h_{n_3-1} 
\end{align}
where $E_{m b}(\cdot )$ is the embedding function, $e()$ is the embedding layer of encoding model $E, h_i \in  
\mathbb{R}^{d_1}$ are learnable vectors, $d_1$ is the embedding dimension of $E$, and $0 \leq i < n_3$. Then the embeddings are fed into the encoding model $E$ and get the hidden representations $m$ of the sentence:

$\boldsymbol{m}=E_{n c}\left(E_{m b}(T(\boldsymbol{x}))\right)$

where $E_{n c}(\cdot)$ represents the hidden layers of $E$. $m \in \mathbb{R}^{d_2}$ refers the hidden representation of [MASK], and $d_2$ is the hidden dimension of $E$.

\textbf{Contrastive Learning}: CPL employs a margin-based contrastive learning (MCL) objective to enhance discriminative feature representation and address overfitting. The MCL loss function is defined as:

Margin-based contrastive learning objective Typically, let $z_i$ be PLMs' output hidden vector after normalization and $s_{i, p}=\boldsymbol{z}_{\boldsymbol{i}} \cdot \boldsymbol{z}_{\boldsymbol{p}}$ denotes positive pair, $s_{i, n}=\boldsymbol{z}_{\boldsymbol{i}} \cdot \boldsymbol{z}_n$ denotes negative pair, the MCL loss can be defined as follows:
$$
\mathcal{L}_{\mathrm{MCL}}(i)=\sum_{p \in P(i)} \log \frac{\exp \left(\alpha_{i, p} \cdot s_{i, p} / \tau\right)}{\mathcal{Z}(i)},
$$
where $P(i)$ denotes the positive set with $i, \tau$ is the temperature constant and $\mathcal{Z}(i)$ is as follows:

\begin{equation}
% \begin{aligned}
    \mathcal{Z}(i)=\sum_{p \in P(i)} \exp \left(\alpha_{i, p} \frac{s_{i, p}}{\tau}\right) \\ +\sum_{n \in N(i)} \exp \left(\alpha_{i, n} \frac{s_{i, n}}{\tau}\right) 
% \end{aligned}
\end{equation}

where $N(i)$ is the negative set with $i, \alpha_{i, p}$ and $\alpha_{i, n}$ are relaxation factors that control the relaxation of the decision boundaries.
$$
\alpha_{i, p}=m+k \cdot s_{i, p}, \alpha_{i, n}=1-m+k \cdot s_{i, n}
$$
where $k$ is normalization constant depends on $s_{i, p}$ and $s_{i, n}, m$ is the margin factor which expects $k$. $s_{i, p}>1-m$ and $k \cdot s_{i, n}<m$.

This objective function prioritizes hard samples, leading to a more uniform feature distribution and mitigating catastrophic forgetting.

\textbf{Memory Augmentation}: After training on the current task, representative samples are selected and stored in memory. Subsequently, CPL utilizes a Large Language Model (LLM), specifically ChatGPT, guided by crafted prompts, to generate diverse samples. These augmented samples are then used in memory replay to reinforce learned knowledge and further combat overfitting.

\textbf{Relation Prediction}: During testing, CPL utilizes a Nearest-Class-Mean (NCM) classifier. This approach leverages the discriminative feature distribution obtained from contrastive training and is well-suited for incremental-class problems.

In conclusion, the CPL framework leverages prompt learning, contrastive learning, and LLM-based memory augmentation to address catastrophic forgetting and overfitting in CFRE, achieving state-of-the-art results on benchmark datasets.
